# Supplementary material for: HIBRIDS: Attention with Hierarchical Biases for Structure-aware Long Document Summarization
Source: arXiv:2203.10741 source file (2022-03-21)
Supplement: Supplementary file 7 [file appendix_E_sample_output.tex]

%auto-ignore
\section{Sample Output}

We show more outputs by \model-\textsc{Enc} on QSGen-Hier in Table~\ref{tab:sample_output}.
